# Supplementary material for: DSV: An Alignment Validation Loss for Self-supervised Outlier Model Selection
Source: arXiv:2307.06534 source file (2023-07-13)
Supplement: Supplementary file 1 [file 110appendix.tex]

\section{Datasets}

Datasets statistics are given as Table \ref{tab:datasets}.

\begin{table}
\setlength\tabcolsep{6pt}
\caption{
    Dataset statistics.
    The first two groups are from MVTec (Textures and Objects, respectively), where the last corresponds to MPDD.
}
\centering
\begin{tabular}{l|rrr}
    \toprule
    \textbf{Task} & \textbf{$|\trnData|$} & \textbf{$|\testDataN|$} & \textbf{$|\testDataA|$} \\
    \midrule
    Carpet & 280 & 28 & 97 \\
    Grid & 264 & 21 & 170 \\
    Leather & 245 & 32 & 99 \\
    Tile & 230 & 33 & 86 \\
    Wood & 247 & 19 & 168 \\
    \midrule
    Bottle & 209 & 20 & 68 \\
    Cable & 224 & 58 & 151 \\
    Capsule & 219 & 23 & 114 \\
    Hazelnut & 391 & 40 & 136 \\
    Metal Nut & 220 & 22 & 132 \\
    Pill & 267 & 26 & 245 \\
    Screw & 320 & 41 & 135 \\
    Toothbrush & 60 & 12 & 66 \\
    Transistor & 213 & 60 & 44 \\
    Zipper & 240 & 32 & 177 \\
    \midrule
    Bracket Black & 289 & 32 & 47 \\
    Bracket Brown & 185 & 26 & 51 \\
    Bracket White & 110 & 30 & 30 \\
    Connector & 128 & 30 & 14 \\
    Metal Plate & 54 & 26 & 71 \\
    Tubes & 122 & 32 & 69 \\
    \bottomrule
\end{tabular}    
\label{tab:datasets}
\end{table}

\newpage
\section{Full Experimental Results}

Tables \ref{tab:accuracy-full-1} and \ref{tab:accuracy-full-2} show the detection AUC on individual tasks, which are used to generate the results in the main paper.

\begin{table}
    \setlength\tabcolsep{5pt}
    \centering
    \caption{
        Detection AUC on (top) CutOut and (bottom) CutAvg.
    }
\resizebox{\textwidth}{!}{
\begin{tabular}{l|cc|ccc|ccc|c}
	\toprule
	Task & Avg. & Rand. & Base & MMD & STD & MC & SEL & HITS & \textbf{\method} \\
	\midrule
	bottle & 0.942 & 0.872 & 0.956 & 0.956 & 0.942 & 0.939 & 0.956 & 0.956 & 0.963 \\
	cable & 0.682 & 0.534 & 0.719 & 0.648 & 0.750 & 0.782 & 0.750 & 0.782 & 0.782 \\
	capsule & 0.644 & 0.669 & 0.673 & 0.701 & 0.680 & 0.652 & 0.652 & 0.662 & 0.657 \\
	carpet & 0.484 & 0.652 & 0.345 & 0.242 & 0.397 & 0.510 & 0.344 & 0.345 & 0.815 \\
	grid & 0.565 & 0.904 & 0.556 & 0.660 & 0.655 & 0.546 & 0.540 & 0.602 & 0.740 \\
	hazelnut & 0.855 & 0.893 & 0.861 & 0.861 & 0.822 & 0.910 & 0.873 & 0.946 & 0.946 \\
	leather & 0.758 & 0.745 & 0.877 & 0.877 & 0.546 & 0.818 & 0.720 & 0.886 & 0.942 \\
	metal nut & 0.572 & 0.631 & 0.563 & 0.563 & 0.565 & 0.513 & 0.513 & 0.563 & 0.563 \\
	pill & 0.752 & 0.694 & 0.756 & 0.756 & 0.797 & 0.756 & 0.772 & 0.855 & 0.855 \\
	screw & 0.124 & 0.451 & 0.265 & 0.265 & 0.145 & 0.054 & 0.054 & 0.044 & 0.428 \\
	tile & 0.761 & 0.869 & 0.632 & 0.632 & 0.694 & 0.813 & 0.813 & 0.731 & 0.776 \\
	toothbrush & 0.972 & 0.872 & 0.956 & 0.972 & 0.981 & 0.978 & 0.978 & 0.981 & 0.917 \\
	transistor & 0.784 & 0.707 & 0.712 & 0.712 & 0.831 & 0.808 & 0.807 & 0.746 & 0.814 \\
	wood & 0.889 & 0.904 & 0.928 & 0.928 & 0.907 & 0.918 & 0.897 & 0.897 & 0.956 \\
	zipper & 0.796 & 0.905 & 0.812 & 0.778 & 0.785 & 0.763 & 0.740 & 0.724 & 0.926 \\
	bracket black & 0.704 & 0.729 & 0.685 & 0.685 & 0.633 & 0.738 & 0.723 & 0.738 & 0.723 \\
	bracket brown & 0.877 & 0.844 & 0.900 & 0.900 & 0.836 & 0.781 & 0.781 & 0.877 & 0.904 \\
	bracket white & 0.804 & 0.818 & 0.819 & 0.788 & 0.817 & 0.639 & 0.508 & 0.721 & 0.733 \\
	connector & 0.998 & 0.967 & 0.993 & 0.993 & 0.998 & 1.000 & 1.000 & 0.998 & 1.000 \\
	metal plate & 0.930 & 0.952 & 0.800 & 0.800 & 0.848 & 0.861 & 0.861 & 0.861 & 0.977 \\
	tubes & 0.623 & 0.688 & 0.749 & 0.721 & 0.884 & 0.957 & 0.977 & 0.980 & 0.666 \\
	\bottomrule
\end{tabular}
}

\vspace{2mm}

\resizebox{\textwidth}{!}{
\begin{tabular}{l|cc|ccc|ccc|c}
	\toprule
	Task & Avg. & Rand. & Base & MMD & STD & MC & SEL & HITS & \textbf{\method} \\
	\midrule
	bottle & 0.921 & 0.917 & 0.913 & 0.913 & 0.921 & 0.930 & 0.913 & 0.919 & 0.900 \\
	cable & 0.701 & 0.593 & 0.582 & 0.572 & 0.739 & 0.668 & 0.668 & 0.818 & 0.716 \\
	capsule & 0.694 & 0.684 & 0.686 & 0.703 & 0.708 & 0.714 & 0.703 & 0.724 & 0.639 \\
	carpet & 0.447 & 0.585 & 0.341 & 0.253 & 0.373 & 0.292 & 0.292 & 0.292 & 0.692 \\
	grid & 0.542 & 0.977 & 0.662 & 0.576 & 0.387 & 0.464 & 0.466 & 0.466 & 0.950 \\
	hazelnut & 0.792 & 0.826 & 0.721 & 0.777 & 0.790 & 0.814 & 0.814 & 0.801 & 0.821 \\
	leather & 0.654 & 0.752 & 0.552 & 0.552 & 0.687 & 0.675 & 0.675 & 0.530 & 0.811 \\
	metal nut & 0.655 & 0.932 & 0.574 & 0.458 & 0.870 & 0.700 & 0.576 & 0.748 & 0.838 \\
	pill & 0.755 & 0.784 & 0.822 & 0.822 & 0.793 & 0.780 & 0.780 & 0.784 & 0.862 \\
	screw & 0.222 & 0.582 & 0.138 & 0.200 & 0.241 & 0.138 & 0.138 & 0.158 & 0.223 \\
	tile & 0.725 & 0.921 & 0.794 & 0.794 & 0.598 & 0.819 & 0.814 & 0.814 & 0.842 \\
	toothbrush & 0.968 & 0.978 & 0.886 & 0.972 & 0.994 & 0.994 & 0.994 & 0.994 & 0.864 \\
	transistor & 0.797 & 0.739 & 0.800 & 0.680 & 0.812 & 0.805 & 0.805 & 0.827 & 0.812 \\
	wood & 0.899 & 0.944 & 0.923 & 0.860 & 0.888 & 0.923 & 0.923 & 0.954 & 0.946 \\
	zipper & 0.824 & 0.971 & 0.850 & 0.747 & 0.856 & 0.856 & 0.856 & 0.856 & 0.940 \\
	bracket black & 0.691 & 0.685 & 0.668 & 0.614 & 0.633 & 0.752 & 0.752 & 0.691 & 0.692 \\
	bracket brown & 0.839 & 0.798 & 0.893 & 0.894 & 0.891 & 0.830 & 0.862 & 0.830 & 0.851 \\
	bracket white & 0.809 & 0.794 & 0.783 & 0.724 & 0.879 & 0.854 & 0.854 & 0.702 & 0.797 \\
	connector & 0.994 & 0.931 & 1.000 & 0.995 & 0.988 & 0.998 & 0.993 & 1.000 & 1.000 \\
	metal plate & 0.856 & 1.000 & 0.837 & 0.837 & 0.843 & 0.894 & 0.894 & 0.790 & 0.865 \\
	tubes & 0.741 & 0.768 & 0.724 & 0.589 & 0.746 & 0.861 & 0.861 & 0.893 & 0.866 \\
	\bottomrule
\end{tabular}
}
\label{tab:accuracy-full-1}
\end{table}

\begin{table}
    \setlength\tabcolsep{5pt}
    \centering
    \caption{
        Detection AUC on (top) CutDiff and (bottom) CutPaste.
    }
\resizebox{\textwidth}{!}{
\begin{tabular}{l|cc|ccc|ccc|c}
	\toprule
	Task & Avg. & Rand. & Base & MMD & STD & MC & SEL & HITS & \textbf{\method} \\
	\midrule
	bottle & 0.924 & 0.907 & 0.925 & 0.925 & 0.945 & 0.945 & 0.945 & 0.935 & 0.904 \\
	cable & 0.688 & 0.756 & 0.663 & 0.582 & 0.740 & 0.792 & 0.792 & 0.763 & 0.792 \\
	capsule & 0.692 & 0.678 & 0.706 & 0.706 & 0.665 & 0.712 & 0.664 & 0.706 & 0.726 \\
	carpet & 0.500 & 0.375 & 0.308 & 0.335 & 0.529 & 0.360 & 0.360 & 0.529 & 0.708 \\
	grid & 0.595 & 0.513 & 0.548 & 0.548 & 0.436 & 0.566 & 0.566 & 0.766 & 0.810 \\
	hazelnut & 0.834 & 0.622 & 0.782 & 0.782 & 0.828 & 0.876 & 0.760 & 0.838 & 0.909 \\
	leather & 0.766 & 0.581 & 0.949 & 0.949 & 0.951 & 0.691 & 0.691 & 0.909 & 0.964 \\
	metal nut & 0.601 & 0.626 & 0.547 & 0.547 & 0.568 & 0.591 & 0.568 & 0.512 & 0.682 \\
	pill & 0.755 & 0.846 & 0.800 & 0.765 & 0.797 & 0.795 & 0.795 & 0.787 & 0.756 \\
	screw & 0.144 & 0.027 & 0.178 & 0.178 & 0.027 & 0.025 & 0.025 & 0.064 & 0.178 \\
	tile & 0.708 & 0.628 & 0.750 & 0.750 & 0.609 & 0.811 & 0.865 & 0.811 & 0.820 \\
	toothbrush & 0.972 & 0.994 & 0.947 & 0.947 & 0.994 & 0.989 & 0.989 & 0.942 & 0.994 \\
	transistor & 0.783 & 0.791 & 0.793 & 0.726 & 0.727 & 0.811 & 0.845 & 0.845 & 0.772 \\
	wood & 0.884 & 0.913 & 0.944 & 0.914 & 0.951 & 0.925 & 0.925 & 0.951 & 0.939 \\
	zipper & 0.823 & 0.796 & 0.818 & 0.818 & 0.791 & 0.807 & 0.807 & 0.791 & 0.913 \\
	bracket black & 0.683 & 0.649 & 0.683 & 0.631 & 0.707 & 0.707 & 0.707 & 0.664 & 0.805 \\
	bracket brown & 0.881 & 0.890 & 0.840 & 0.894 & 0.865 & 0.829 & 0.851 & 0.861 & 0.897 \\
	bracket white & 0.813 & 0.783 & 0.851 & 0.851 & 0.807 & 0.566 & 0.566 & 0.777 & 0.791 \\
	connector & 0.998 & 0.993 & 1.000 & 0.990 & 0.998 & 1.000 & 0.998 & 0.988 & 1.000 \\
	metal plate & 0.930 & 0.939 & 0.871 & 0.871 & 0.932 & 0.901 & 0.901 & 0.888 & 0.975 \\
	tubes & 0.623 & 0.614 & 0.613 & 0.613 & 0.747 & 0.980 & 0.932 & 0.980 & 0.691 \\
	\bottomrule
\end{tabular}
}

\vspace{2mm}

\resizebox{\textwidth}{!}{
\begin{tabular}{l|cc|ccc|ccc|c}
	\toprule
	Task & Avg. & Rand. & Base & MMD & STD & MC & SEL & HITS & \textbf{\method} \\
	\midrule
	bottle & 0.964 & 0.991 & 0.967 & 0.967 & 1.000 & 0.987 & 1.000 & 0.967 & 0.980 \\
	cable & 0.690 & 0.684 & 0.560 & 0.603 & 0.805 & 0.903 & 0.895 & 0.939 & 0.805 \\
	capsule & 0.807 & 0.866 & 0.701 & 0.701 & 0.715 & 0.880 & 0.811 & 0.882 & 0.882 \\
	carpet & 0.497 & 0.772 & 0.289 & 0.377 & 0.504 & 0.555 & 0.555 & 0.555 & 0.840 \\
	grid & 0.854 & 0.994 & 0.634 & 0.986 & 0.999 & 0.998 & 0.997 & 0.991 & 0.986 \\
	hazelnut & 0.708 & 0.690 & 0.571 & 0.629 & 0.750 & 0.760 & 0.749 & 0.720 & 0.760 \\
	leather & 0.756 & 0.969 & 0.822 & 0.934 & 0.559 & 0.756 & 0.624 & 0.875 & 0.934 \\
	metal nut & 0.723 & 0.761 & 0.696 & 0.696 & 0.603 & 0.841 & 0.687 & 0.886 & 0.909 \\
	pill & 0.784 & 0.766 & 0.799 & 0.799 & 0.751 & 0.762 & 0.762 & 0.799 & 0.903 \\
	screw & 0.579 & 0.857 & 0.179 & 0.179 & 0.454 & 0.750 & 0.700 & 0.602 & 0.750 \\
	tile & 0.725 & 0.826 & 0.436 & 0.527 & 0.896 & 0.961 & 0.961 & 0.749 & 0.961 \\
	toothbrush & 0.954 & 0.903 & 0.986 & 0.989 & 0.964 & 0.989 & 0.994 & 0.989 & 0.958 \\
	transistor & 0.778 & 0.688 & 0.606 & 0.945 & 0.811 & 0.960 & 0.939 & 0.939 & 0.924 \\
	wood & 0.890 & 0.887 & 0.902 & 0.934 & 0.970 & 0.934 & 0.902 & 0.954 & 0.874 \\
	zipper & 0.903 & 0.970 & 0.737 & 0.737 & 0.994 & 0.995 & 0.995 & 0.950 & 0.995 \\
	bracket black & 0.724 & 0.783 & 0.637 & 0.637 & 0.696 & 0.701 & 0.754 & 0.725 & 0.725 \\
	bracket brown & 0.890 & 0.837 & 0.925 & 0.925 & 0.977 & 0.859 & 0.859 & 0.977 & 0.850 \\
	bracket white & 0.838 & 0.924 & 0.698 & 0.780 & 0.977 & 0.851 & 0.630 & 0.644 & 0.977 \\
	connector & 0.984 & 0.952 & 0.962 & 0.940 & 0.993 & 1.000 & 1.000 & 1.000 & 0.940 \\
	metal plate & 0.782 & 0.836 & 0.756 & 0.876 & 0.863 & 0.880 & 0.880 & 0.880 & 0.848 \\
	tubes & 0.710 & 0.707 & 0.715 & 0.715 & 0.898 & 0.775 & 0.732 & 0.837 & 0.752 \\
	\bottomrule
\end{tabular}
}
\label{tab:accuracy-full-2}
\end{table}
